# Supplementary material for: Q-learning with online random forests
Source: arXiv:2204.03771 source file (2022-04-07)
Supplement: Supplementary file 1 [file supmat.pdf]

---

# $Q$ -LEARNING WITH ONLINE RANDOM FORESTS (SUPPLEMENTARY MATERIAL)

---

✉ Joosung Min    ✉ Lloyd T. Elliott

Department of Statistics and Actuarial Science  
Simon Fraser University, British Columbia, Canada  
joosung\_min@sfu.ca, lloyd\_elliott@sfu.ca

## 1 Algorithms for RL-ORF

---

### Algorithm 1 $Q$ -Learning with Online Trees

---

**Require:** Replay memory to capacity  $N_{\text{mem}}$ , minibatch size:  $N_{\text{min}}$ , temporal knowledge weighting rate:  $\varphi$ , episode at which to expand ensemble size:  $\delta$ , maximum ensemble size:  $|M_{\text{max}}|$ .

```
1: for episode  $i$  in  $1 : E$  do
2:   for time step  $t$  in  $1 : T$  do
3:     Select  $a_t = \text{nextAction}(s_t)$  # According to Algorithm 2.
4:     Execute  $a_t$  and obtain tuple  $e_t = (s_t, a_t, r_t, s_{t+1})$ , store it in the replay memory
5:     Randomly sample minibatch of  $(s_\ell, a_\ell, r_\ell, s_{\ell+1})$  from the replay memory
6:     Set  $y_\ell = \begin{cases} r_\ell + \gamma * \max_a \hat{Q}(s_{\ell+1}, a_\ell) & \text{if } s_{\ell+1} \text{ is not terminal} \\ r_\ell & \text{if } s_{\ell+1} \text{ is terminal} \end{cases}$ 
7:     for tree  $m$  in  $1 : M_{a_j}$  do
8:       Draw  $c \sim \text{Poisson}(1)$ 
9:       if  $c > 0$  then
10:        for  $k$  in  $1 : c$  do
11:          Set  $\text{age}_m + = 1$ 
12:          Set  $j = \text{findLeaf}(s_\ell)$ 
13:           $\text{updateNode}(j, \langle s_\ell, y_\ell \rangle)$ 
14:        end for
15:       else
16:         $\text{updateOOBE}_m$  # According to Algorithm 5
17:       end if
18:     end for
19:     # Perform temporal knowledge weighting on ensemble  $M_{a_\ell}$ 
20:     Randomly select  $m$  from  $M_{a_\ell}$  such that  $\text{age}_m > 1/\varphi$ 
21:     if  $\text{OOBE}_m > c \sim \text{Uniform}(0, 1)$  then
22:       Replace the tree with a new tree with just one node
23:     end if
24:   end for
25:   if  $i = \zeta$  then
26:      $\text{expandTrees}(M, |M_{\text{max}}|)$  # According to Algorithm 4
27:   end if
28: end for
```

---

---

**Algorithm 2** nextAction( $s_t$ )

**Require:** Probability of taking a random action:  $\varepsilon$ , a state observed at time step  $t$ :  $s_t$ , an action space:  $A$ , an ensemble of trees:  $M$ .

- 1: Draw  $c \sim \text{Uniform}(0, 1)$
  - 2: **if**  $c < \varepsilon$  **then**
  - 3:     **return**  $a_{t+1} = \text{random action from } \mathcal{A}$
  - 4: **else**
  - 5:     **return**  $a_{t+1} = \text{argmax} (M_1(s_{t+1}), \dots, M_{|A|}(s_{t+1}))$
  - 6: **end if**
- 

---

**Algorithm 3** createChild( $\mathbf{p}_{j \cdot h}$ )

**Require:** The number of explanatory variables:  $K$ , the state attributes in the environment =  $\{z_1, \dots, z_K\}$ .

- 1: Set  $\mathbf{p}_{j+1} = \mathbf{p}_{j \cdot h}$   
   # Apply partial randomness in split point selection.
  - 2: Select  $K$  split points  $\{\theta_1, \dots, \theta_K\}$ , where  $\theta_i \sim \text{Uniform}(\min(z_i), \max(z_i)) \forall i$
  - 3: Construct a set of tests  $\mathbf{H}_j = \{h_1, \dots, h_K\}$ , where  $h_i = (z_i, \theta_i) \forall i$
- 

---

**Algorithm 4** expandTrees( $M, |M_{max}|$ )

**Require:** Ensemble of trees:  $M$ , the initial size of ensemble:  $|M_{init}|$ , the maximum size of ensemble:  $|M_{max}|$ .

- 1:  $m_{best} = \{m | m \in M, \text{OOBE}_m = \min_{m \in M} \text{OOBE}_m\}$
  - 2: **for**  $i$  in  $|M_{init}| + 1 : |M_{max}|$  **do**
  - 3:      $M = \text{append}(M, m_{best})$
  - 4: **end for**
- 

---

**Algorithm 5** updateOOBE( $\langle x, y \rangle$ )

**Require:** Tree index:  $m$

**Require:** Training example:  $\langle x, y \rangle$

**Require:** Number of training samples the tree has observed:  $age_m$

- 1:  $y_{pred} = m(x)$
  - 2: **if**  $y \neq y_{pred}$  **then**
  - 3:      $error_m + = 1$
  - 4:      $\text{OOBE}_m = error_m / age_m$
  - 5: **end if**
-

## 2 Experiment: Blackjack

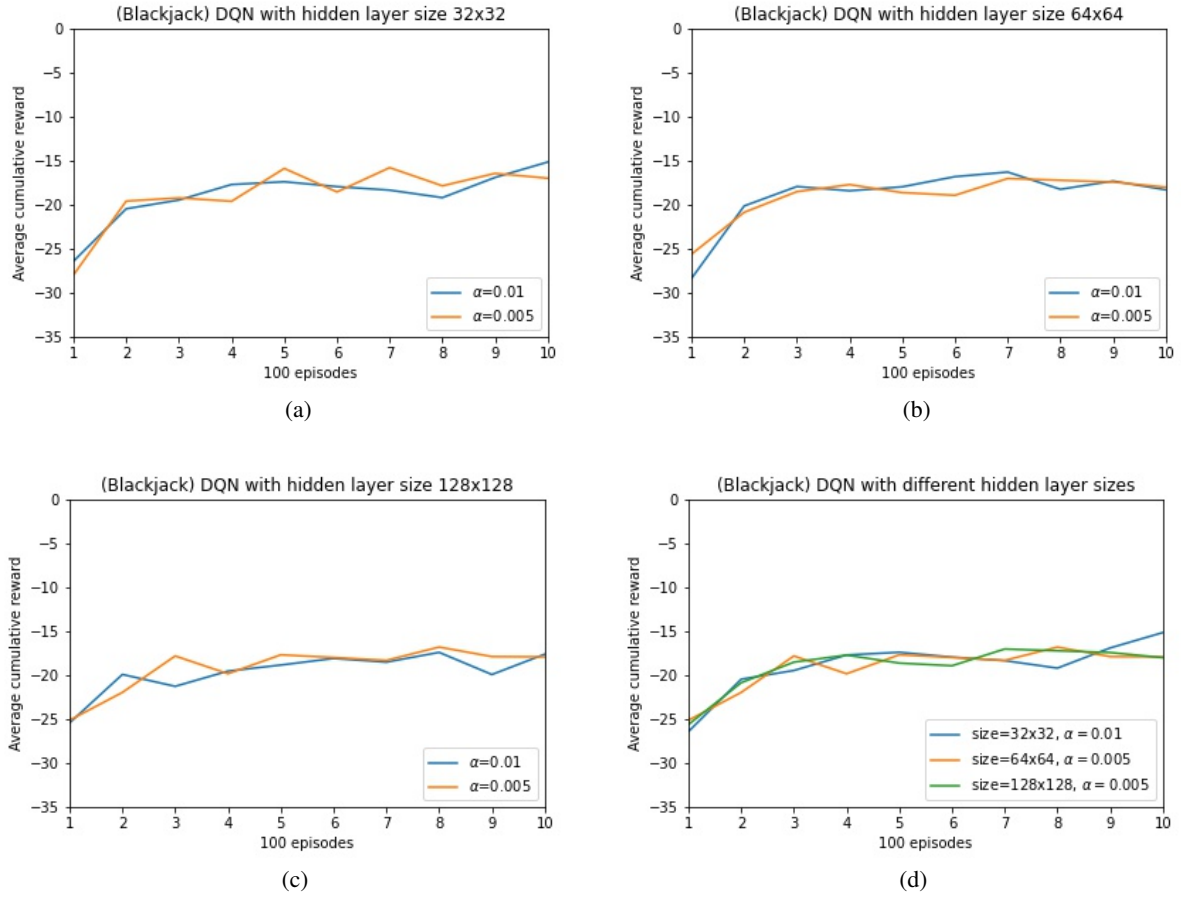

Figure 1: Performance of DQNs with different hidden layer sizes (given in legend) and learning rates ( $\alpha$ ) in the blackjack gym. The size 128x128 performed the best at episode 1,000.  $\alpha$  indicates learning rate.

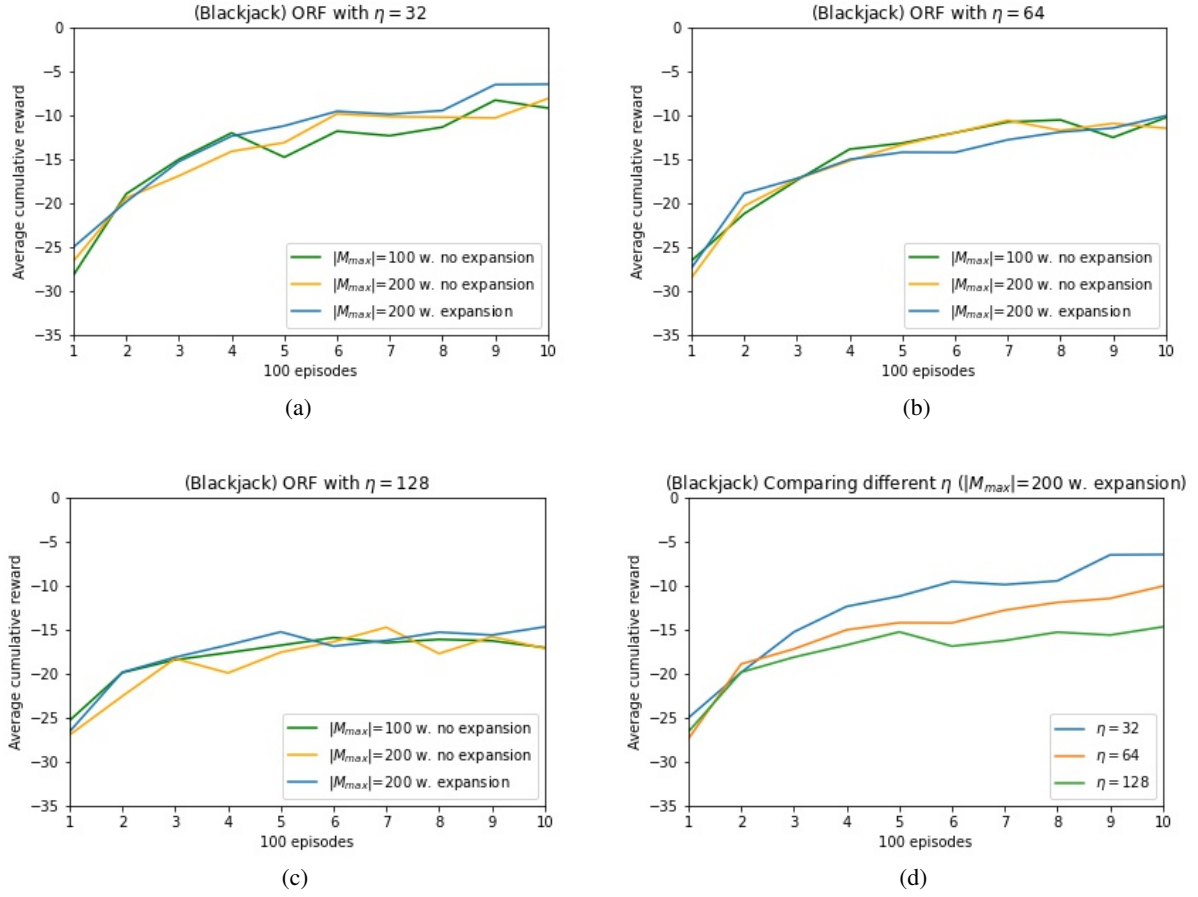

Figure 2: Performance of RL-ORF with different  $\eta$  (samples observed per terminal node), ensemble sizes, and whether to expand ensemble size. RL-ORF with  $\eta = 32$ ,  $|M_{max}| = 200$  and *with* expansion performed the best at episode 1,000.

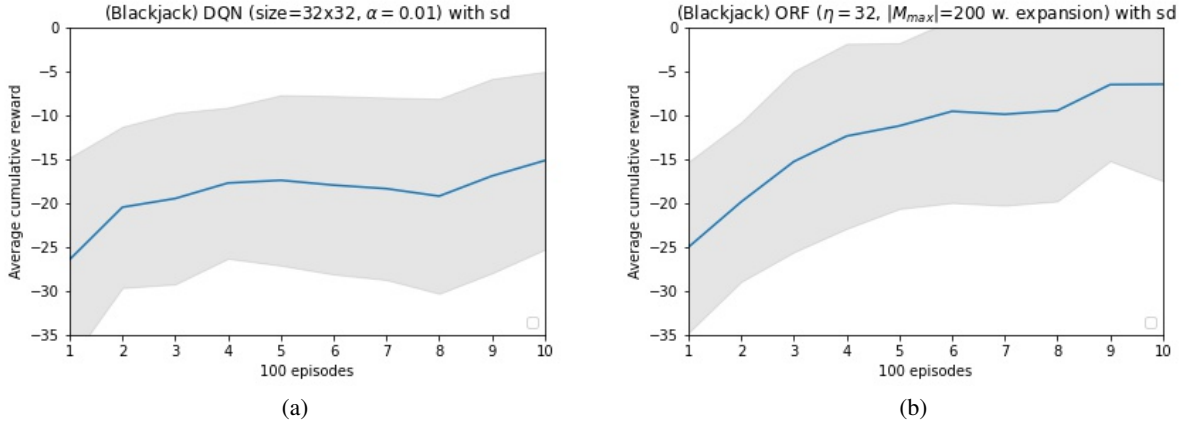

Figure 3: Performance of the best DQN and RL-ORF with their error regions. The error regions are standard errors on 100 random restarts. RL-ORF outperformed DQN at episode 1,000.

| Shapiro-Wilk Test |                                   |         |           |            |                  |
|-------------------|-----------------------------------|---------|-----------|------------|------------------|
| Approx.           | Parameters                        | Episode | Statistic | $p$ -value | Conclusion       |
| DQN               | size=32x32, $\alpha=0.01$         | 300     | 0.970     | 0.886      | Cannot reject H0 |
| DQN               | size=32x32, $\alpha=0.01$         | 1000    | 0.921     | 0.330      | Cannot reject H0 |
| ORF               | $\eta=32$ , $ M_{max} =200$ , exp | 300     | 0.979     | 0.113      | Cannot reject H0 |
| ORF               | $\eta=32$ , $ M_{max} =200$ , exp | 1000    | 0.976     | 0.060      | Cannot reject H0 |

Table 1: (Blackjack) Shapiro-Wilk normality test performed on the average rewards at episodes 300 and 1,000 with significance level 0.05. The  $p$ -values indicate that the average rewards are normally distributed.

| t-Test  |           |                   |            |
|---------|-----------|-------------------|------------|
| Episode | Statistic | $p$ -value        | Conclusion |
| 300     | -0.428    | 0.665             | Accept H0  |
| 1000    | 4.249     | $2.271 * 10^{-5}$ | Reject H0  |

Table 2: (Blackjack) A one-sided t-test to compare the mean rewards of DQN and RL-ORF. The  $p$ -values suggest that there is statistical evidence that the mean average reward from RL-ORF is greater than the mean average reward from DQN at episode 1,000, but not at 300 at a significance level = 0.05.

### 3 Experiment: Inverted pendulum

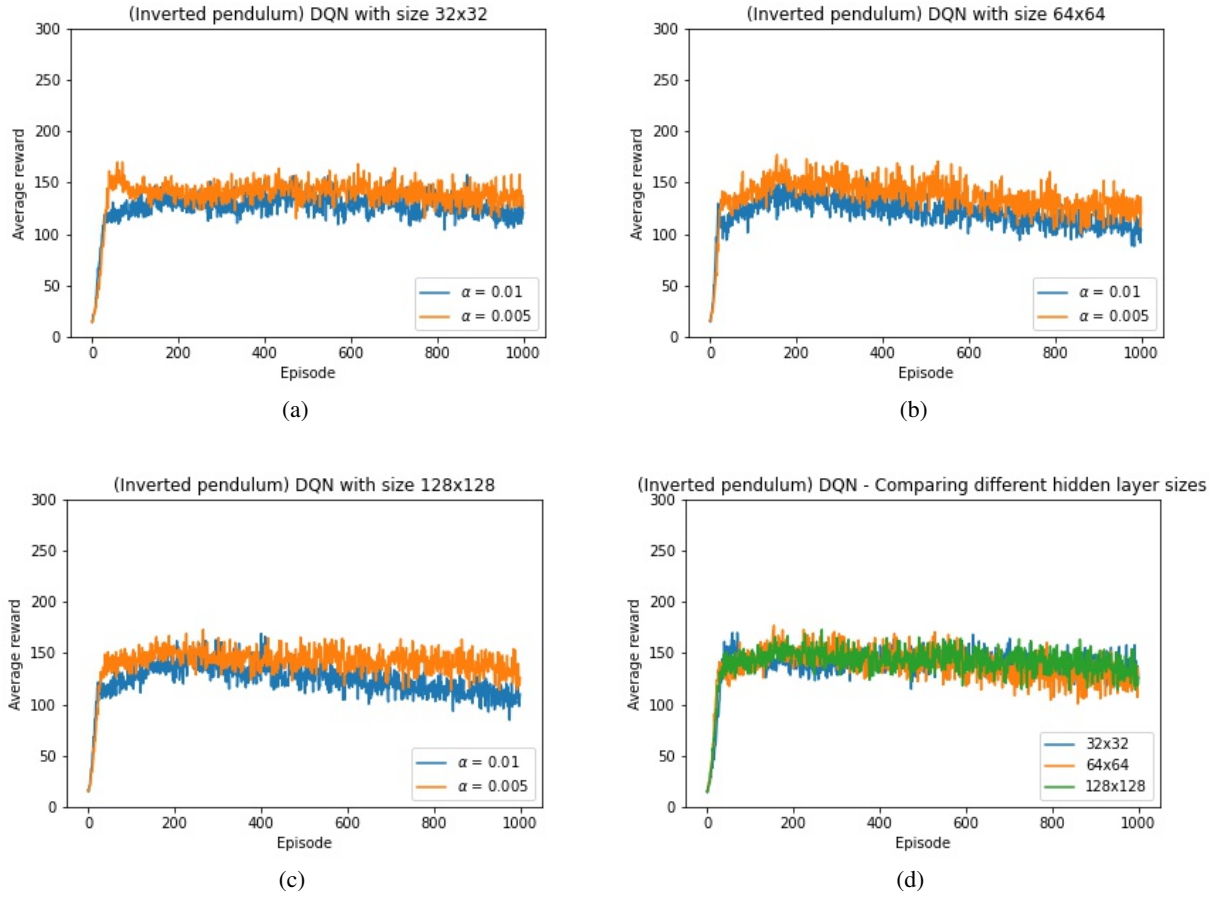

Figure 4: Performances of DQNs with different hidden layer sizes and learning rates in the inverted pendulum environment. DQN with hidden layer size 128x128 and  $\alpha = 0.005$  performed the best.

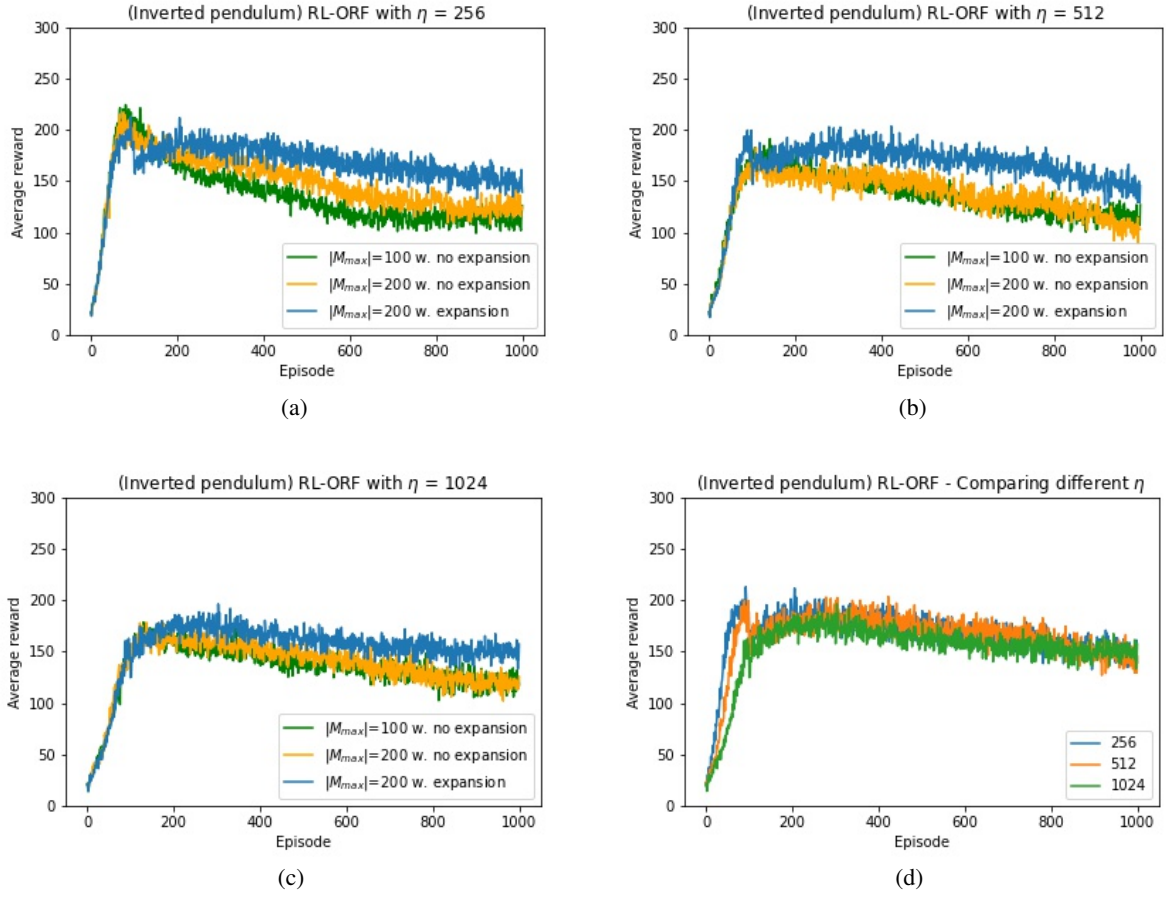

Figure 5: Performances of RL-ORF with different  $\eta$  (samples observed per terminal node), ensemble sizes, and whether to expand ensemble size. RL-ORF with  $\eta = 256$ ,  $|M_{max}| = 200$  with expansion performed the best at episode 1,000.

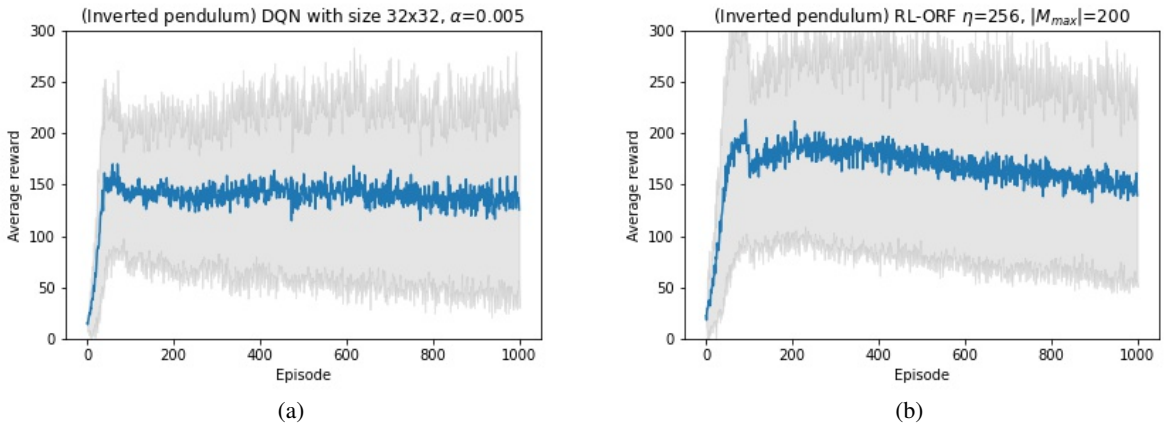

Figure 6: Performances of the best DQN and RL-ORF with their error regions. The error regions are standard errors on 100 random restarts. RL-ORF outperformed DQN at episode 1,000.

| Shapiro-Wilk Test |                                          |         |           |                   |            |
|-------------------|------------------------------------------|---------|-----------|-------------------|------------|
| Approx.           | Parameters                               | Episode | Statistic | $p$ -value        | Conclusion |
| ORF               | $\eta=256,  M_{max} =200, \text{Exp}$    | 300     | 0.803     | $2.97 * 10^{-10}$ | Reject H0  |
| ORF               | $\eta=256,  M_{max} =200, \text{Exp}$    | 1000    | 0.809     | $4.68 * 10^{-10}$ | Reject H0  |
| ORF               | $\eta=256,  M_{max} =200, \text{no Exp}$ | 300     | 0.794     | $1.89 * 10^{-10}$ | Reject H0  |
| ORF               | $\eta=256,  M_{max} =200, \text{no Exp}$ | 1000    | 0.788     | $1.26 * 10^{-10}$ | Reject H0  |

Table 3: ( $\eta = 256, |M_{max}| = 200$  w. expansion vs. no expansion) The large  $p$ -values from Shapiro-Wilk normality test suggest that the data are not normally distributed.

| Mann-Whitney U Test |           |            |                  |
|---------------------|-----------|------------|------------------|
| Episode             | Statistic | $p$ -value | Conclusion       |
| 300                 | 5557.0    | 0.068      | Cannot reject H0 |
| 1000                | 5654.0    | 0.042      | Reject H0        |

Table 4: ( $\eta = 256, |M_{max}| = 200$  w. expansion vs. no expansion) The  $p$ -values from Mann-Whitney U-test indicate that the null hypothesis that the mean from RL-ORF with expansion is greater than the other cannot be rejected with a significance level of 0.05 at episode 300, but can be rejected at 1,000.

| Shapiro-Wilk Test |                                       |         |           |                   |            |
|-------------------|---------------------------------------|---------|-----------|-------------------|------------|
| Approx.           | Parameters                            | Episode | Statistic | $p$ -value        | Conclusion |
| DQN               | size=128x128, $\alpha=0.005$          | 300     | 0.813     | $6.53 * 10^{-10}$ | Reject H0  |
| DQN               | size=128x128, $\alpha=0.005$          | 1000    | 0.877     | $1.34 * 10^{-7}$  | Reject H0  |
| ORF               | $\eta=256,  M_{max} =200, \text{exp}$ | 300     | 0.803     | $2.97 * 10^{-10}$ | Reject H0  |
| ORF               | $\eta=256,  M_{max} =200, \text{exp}$ | 1000    | 0.809     | $4.68 * 10^{-10}$ | Reject H0  |

Table 5: (RL-ORF vs. DQN) A Shapiro-Wilk test shows that the data are not normally distributed.

| Mann-Whitney U Test |           |            |            |
|---------------------|-----------|------------|------------|
| Episode             | Statistic | $p$ -value | Conclusion |
| 300                 | 6464.5    | 0.0002     | Reject H0  |
| 1000                | 5965.0    | 0.009      | Reject H0  |

Table 6: (RL-ORF vs. DQN). Small  $p$ -values from the Mann-Whitney U-test indicate that there is statistical evidence that the mean rewards from RL-ORF are greater than the mean rewards from DQN.

## 4 Experiment: Lunar Lander

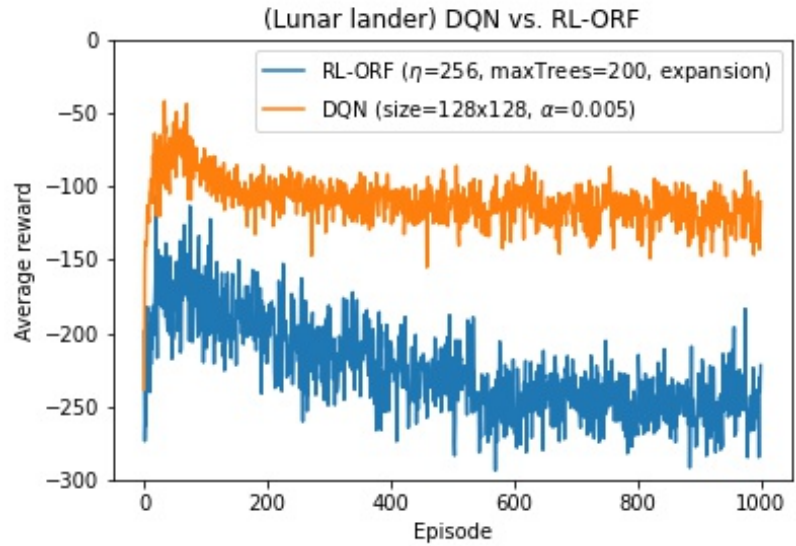

Figure 7: Average reward per episode on the lunar lander environment. Neither DQN nor RL-ORF performed well. Both models demonstrate catastrophic forgetting. DQN’s average reward was higher throughout the episodes.
